# Supplementary material for: Pruned Pivot: Correlation Clustering Algorithm for Dynamic, Parallel, and Local Computation Models
Source: arXiv:2402.15668 source file (2024-06-14)
Supplement: Supplementary file 1 [file appendix.tex]

\appendix
\section{Proof of \cref{thm:equivalent}}

Fix an ordering $\pi$ in both algorithms. We prove that for each node $v$, either (1) $v$ is a singleton in \NSPivot and an unlucky node in Pivot, or (2) The pivot and radius of $v$ is the same in both algorithms.

We prove this via induction on $\pi(v)$. Suppose that $\pi(v)=1$. In both \textsc{Pivot} and \NSPivot algorithms, $v$ is a pivot with radius $0$. Note that $v$ doesn't query any nodes, so in \NSPivot it is not a singleton, and it is not unlucky (neither width or length unlucky) in \textsc{Pivot}. 

Next suppose that $\pi(v)=i>1$.  %Note that this means for any node $u$ with $\pi(u)<i$, $u$ is a singleton in \NSPivot if and only if it is width or length unlucky in \textsc{Pivot}.
Consider all the neighbors $u$ of $v$ with $\pi(u)<\pi(v)$. By induction hypothesis, either $u$ is a singleton in \NSPivot and unlucky in \textsc{Pivot}, or $u$ has the same pivot and radius in both algorithms.%$p(u)=p_{NS}(u)$ and $radius(u)=radius_{NS}(u)$. 

First we make an observation: In \textsc{Pivot} if $v$ queries an unlucky node $u$, no matter how it is clustered it will become an unlucky node: either $u$ is depth unlucky in which case $v$ is also depth unlucky, or $u$ is width unlucky of generation $g$ in which case $v$ is depth unlucky of generation $g+1$. So we can assume that the algorithm halts when $v$ queries $u$. 

With this observation the processing of node $v$ in \NSPivot and \textsc{Pivot} with depth and width pruning is done in the same way: Going through the neighbors of $v$ in descending order with respect to $\pi$, both algorithms query each neighbor $u$ of $v$ with $\pi(u)<\pi(v)$ until one of these cases happen:

(1) $u$ is a pivot, in which case it is pivot in both algorithms.

(2) $u$ is an unlucky node in \textsc{Pivot} and a singleton in \NSPivot in which case $v$ is an unlucky node in \textsc{Pivot} (by the above observation) and a singleton in \NSPivot.

(3) $k$ nodes have been queried and neither (1) or (2) has happened. In this case in \NSPivot $v$ is a singleton and in \textsc{Pivot} $v$ is a first generation width unlucky node. Note that \textsc{Pivot} might continue query more nodes but it doesn't matter as $v$ is now an unlucky node.

(4) neither (1), (2) or (3) has happened in which case $v$ is a pivot in both algorithms.

Note that in cases (1) and (2), the set of nodes that $v$ queries is the same in both algorithms. Hence the radius and pivot of $v$ are the same in both algorithm. This finishes the proof.
